# Supplementary material for: Efficient Compactions Between Storage Tiers with PrismDB
Source: arXiv:2008.02352 source file (2022-05-25)
Supplement: Supplementary file 1 [file appendix.tex]

\appendix
\clearpage
\section{APPENDIX}

\begin{figure}[t!]
	\begin{center}
	{\includegraphics[width=0.65\columnwidth]{paper/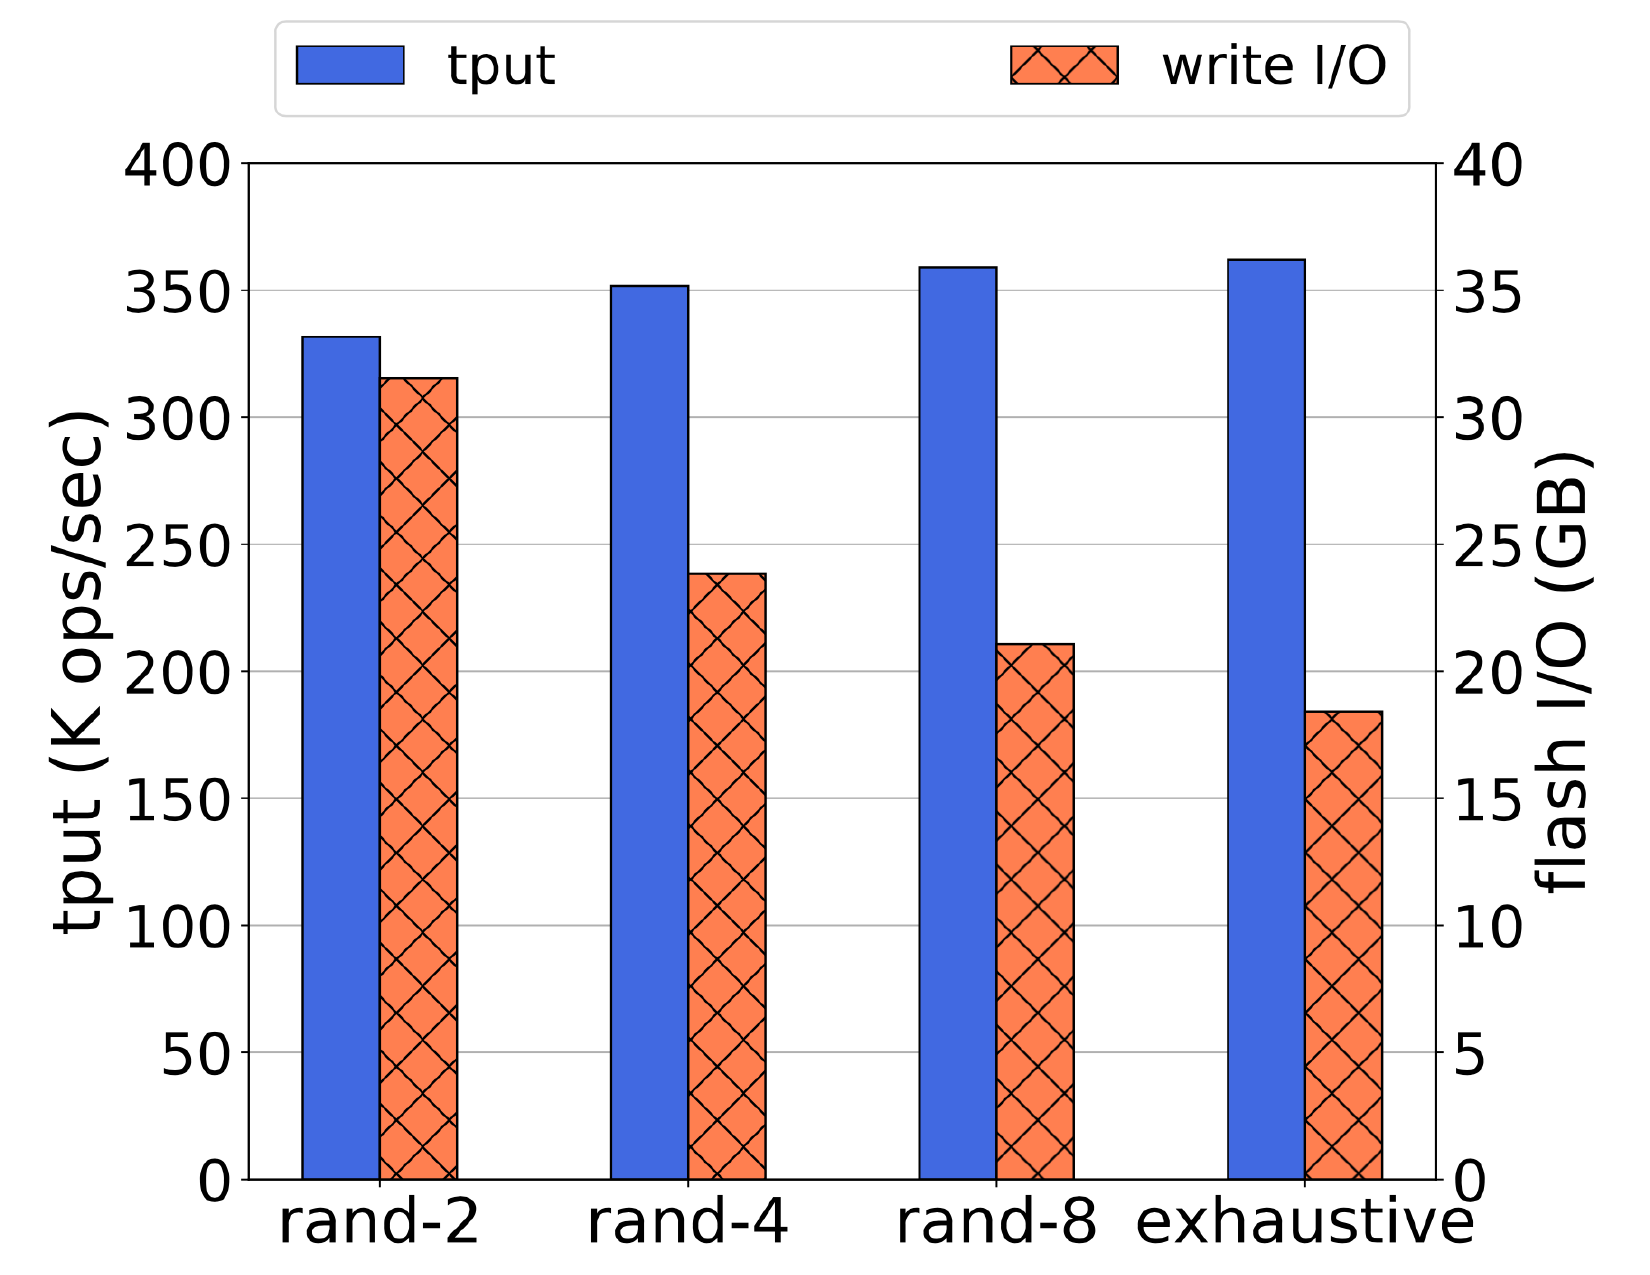}}
	\end{center}
	\caption{Comparison of throughput and flash write I/O between different key range selection algorithms using the approx-$MSC$ policy in \name under YCSB-A zipf 0.99 workload.}
	\label{fig:mig-policy}
\end{figure}

\subsection{Key Range Selection Evaluation}
\label{sec:appendix-key-range-selection}

We evaluate different key-range selection algorithms. 
We compare exhaustive search with a power of k choices algorithm, rand-$k$, that randomly samples $k$ compaction key ranges from all candidates. 
%The more random choices we consider, the closer we are to exhaustive search.
%We compare rand-2, rand-4 and rand-8, and evaluate them with the approx-M metric under YCSB-A.
Figure~\ref{fig:mig-policy} shows their respective throughput and flash write I/Os. All algorithms exhibit similar CPU utilization ($\sim$50\%).
As $k$ increases, flash write I/O gradually drops from 32~GB to 18~GB, approaching the flash I/O of exhaustive search. 
At the same time, throughput increases, because more choices allow \name to select better key range candidates. 
We find power of k choices with $k=8$ to be a reasonable key-range selection algorithm since it gives high throughput while keeping flash write I/O low.
% The approx-$MSC$ metric with rand-8 range selection mechanism yields the best overall throughput (Table~\ref{tab:mig-tput}). 
% We use this combination in \S\ref{sec:eval}.
